# Supplementary material for: The Limits to Learning a Diffusion Model
Source: arXiv:2006.06373 source file (2023-05-23)
Supplement: Supplementary file 1 [file appendix_time_to_peak_v1.tex]

\section{Proofs related to time to peak limit}

\subsection{Proof of Theorem~\ref{thm:deterministic-time}}

%% removed >
\iffalse

Consider the deterministic SIR model \textcolor{teal}{as defined in \ref{}}

\begin{align} \label{eq:ode}
\frac{dS}{dt} &=  - \beta \frac{S}{N} I   &
\frac{dI}{dt} &= \beta \frac{S}{N} I - \gamma I  &
\frac{dR}{dt} &= \gamma I
\end{align}
All quantities are non-negative. 
% $S$ is non-increasing, while $R$ is non-decreasing.

Define $T_1$ to be the time when $N^{2/3}$ individuals have become infected since $t = 0$, i.e. $S(0) - S(T_1) = N^{2/3}$.
Define $T_2$ to be the time when $S(T_2) = \frac{\gamma}{\beta} N$. $T_2$ is the ``peak time'', since $I$ starts to decrease after this point.
Our goal is to show $\frac{T_1}{T_2} \geq \frac{2}{3}$.
We consider the regime where $\beta, \gamma$, and $I(0)$ are fixed, $\beta > \gamma$, and $N \rightarrow \infty$.

\begin{theorem} \label{thm:time_to_peak} Consider the deterministic SIR model, with $\beta, \gamma$, and $I(0)$ fixed, and $\beta > \gamma$. Let $T_1$ to be the time when $N^{2/3}$ individuals have become infected since $t = 0$, i.e. $S(0) - S(T_1) = N^{2/3}$ and $T_2$ to be the time when $S(T_2) = \frac{\gamma}{\beta} N$. $T_2$ is the ``peak time'', since $I$ starts to decrease after this point. Then, as $N \rightarrow \infty$,
\begin{align*}
\lim_{N \rightarrow \infty} \frac{T_1}{T_2} \geq \frac{2}{3}.
\end{align*}
\end{theorem}

\fi
%% removed <

%\subsection{Proof Sketch}
% Our goal is to lower bound $T_1 \gtrsim \frac{2}{3}\log N$ and upper bound $T_2 \lesssim \log N$.

\paragraph{Proof Sketch.} Our goal is to lower bound $T_1$ upper bound $T_2$. One method of constructing lower and upper bounds is to consider the modified set of ODE's from \eqref{eq:sirfluid} where the term $\frac{S}{N}$ is replaced by a constant $\rho$, which allows the ODE's to be solved exactly.
If this constant is larger than $\frac{S}{N}$ (e.g. $\rho = 1$), then the solution to the new ODE's provides a ``faster'' infection process than the original, which in turn results in a lower bound for $T_1$.

We cannot use the exact same technique to upper bound $T_2$. 
To see this, we need to set $\rho$ to be smaller than $S(t)/N$ for all $t \leq T_2$. 
Since $T_2$ is defined as the time when $S(t)/N = \frac{\gamma}{\beta}$, it must be that $\rho = \frac{\gamma}{\beta}$.
However, replacing $\frac{S}{N}$ with $\gb$ in \eqref{eq:sirfluid} results in $\frac{dI}{dt} = \beta \rho I - \gamma I = 0$, providing the trivial lower bound of $I(t)=0\; \forall t$.
Therefore, this technique only provides a meaningful bound when $\rho > \gb$.

Therefore, we break down $T_2$ into $\tone + (T_2 - \tone)$,
where $\tone$ is the time that $S(\tone)/N = \rho_1$ for a specific $\rho_1 > \gb$.
Then, we can use the above method to lower bound $\tone$.
Between the times $\tone$ and $T_2$, exactly $N(\rho_1 - \gb)$ individuals need to become newly infected.  
The rate at which individuals become infected is $-\frac{dS}{dt} = \beta \frac{S}{N} I \geq \beta \gb I(\tone)$ for $t \in [\tone, T_2]$.
Therefore, $T_2 - \tone \geq \frac{N(\rho_1 - \gb)}{\gamma I(\tone)}$.
Combining these results using $\rho_1 = 1 - \frac{1}{\log \log N}$ provides the desired upper bound for $T_2$.

%\subsection{Proof}
\begin{proof}[Proof of Theorem~\ref{thm:deterministic-time}] The crux of the argument is summarised in two smaller results, bounding $T_1$ and $T_2$ respectively.  

\begin{proposition} \label{prop:T1}
There exists a constant $\nu_1$ that only depends on $\beta, \gamma, I(0)$ such that
\begin{align*}
T_1 \geq \frac{2}{3} \frac{1}{\beta - \gamma} \log\left( \nu_1 N\right).
\end{align*}
\end{proposition}

\begin{proposition} \label{prop:T2}
Let $\rho_1 = 1 - \frac{1}{\log \log N}$.
There exist constants $C, \nu_2$ that only depend on $\beta, \gamma, I(0)$ such that 
\begin{align*}
T_2 \leq \frac{1}{\beta \rho_1 - \gamma} \log(\nu_2 N) + \frac{C}{(1-\rho_1)}.
\end{align*}
\end{proposition}

Now, the argument follows directly by taking the limit of the bounds we provide in Propositions~\ref{prop:T1}-\ref{prop:T2}.
\begin{align*}
\lim_{N \rightarrow \infty} \frac{T_2}{T_1} 
&\leq \lim_{N \rightarrow \infty}  \frac{\frac{1}{\beta \rho_1 - \gamma} \log(\nu_2 N) + \frac{C}{(1-\rho_1)}}{\frac{2}{3} \frac{1}{\beta - \gamma} \log\left( \nu_1 N\right)} \\
&= \lim_{N \rightarrow \infty} \frac{3}{2}\left( \frac{\beta - \gamma}{\beta \rho_1 - \gamma}\cdot \frac{\log N + \log \nu_2}{\log N + \log \nu_1} +  \frac{(\beta - \gamma) C \log \log N}{\log (\nu_1 N)} \right) \\
&= \frac{3}{2}
\end{align*}   
\end{proof}

\subsubsection{Proof of Proposition~\ref{prop:T1}}

\begin{proof} [Proof of Proposition~\ref{prop:T1}]

%% removed >
%\iffalse
Define $\tI(t)$ such that $\tI(0) = I(0)$ and $\frac{d\tI}{dt} = (\beta - \gamma) \tI$, implying 
\begin{align}
\tI(t) = I(0) \exp\{ (\beta - \gamma) t\}.
\end{align}
Since $\frac{d\tI}{dt} \geq \frac{dI}{dt}$ for all $t$, $\tI(t) \geq I(t)$ for all $t$.

Then, for all $t$,
\begin{align}
\frac{dS}{dt} = - \beta \frac{S}{N} I 
              &\geq - \beta \tI.
\end{align}
Hence we can write

Using the definition of the deterministic SIR model, we have 
\begin{align}
S(t) 
&\geq S(0) +  \int_{0}^{t} - \beta \tI(t') dt' \\
&=S(0)- \beta  I(0)\int_{0}^{t}  \exp\{ (\beta  - \gamma) t'\} dt' \\
&= S(0)- \frac{\beta  I(0)}{\beta  - \gamma}( \exp\{ (\beta- \gamma) t \} -1)  \\
\end{align}
%% removed <
%\fi

Since $S(0) - S(T_1) = N^{2/3}$, solving for $T_1$ in the inequality above results in 
\begin{align}
T_1 \geq \frac{1}{\beta - \gamma} \log\left( \frac{\beta - \gamma}{\beta I(0)} N^{2/3}\right)
\geq \frac{2}{3} \frac{1}{\beta - \gamma} \log\left( \nu_1 N\right),
\end{align}
for $\nu_1 = \left(\frac{\beta - \gamma}{\beta I(0)}\right)^{3/2}$ as desired.
\end{proof}

\subsubsection{Proof of Proposition~\ref{prop:T2}}
For $\rho \in [0, \frac{\gamma}{\beta}]$, let $t_\rho$ be the time $t$ when $\frac{S(t)}{N} = \rho$.
$\rho$ will represent the fraction of the total population that is susceptible.
Since $\rho \leq \frac{\gamma}{\beta}$, $I$ is increasing for the time period of interest.

Let $\beta > \gamma$, $N$ be fixed. Let $\rho_1 = 1 - \frac{1}{\log \log N}$ and $\rho_2 = \frac{\gamma}{\beta}$.
We assume $N$ is large enough that $\rho_1 > \rho_2$, hence $\tone < \ttwo$.
$T_2 = \ttwo$.

\begin{lemma} \label{lemma1}
For any $\rho \in [0, \frac{\gamma}{\beta}]$, 
% \begin{align}
$I(t_\rho) \geq N(1-\rho)\frac{\beta \rho - \gamma}{\beta \rho}$.
% \end{align}
\end{lemma}

\begin{proof}[Proof of Lemma~\ref{lemma1}]
Fix $\rho$.
At time $t_\rho$, the total number of people infected is $C(t_\rho) = I(t_\rho) + R(t_\rho) = N(1-\rho)$, by definition. 
At any time $t \leq t_\rho$, the rate of increase in $I$ is $\frac{\beta \frac{S(t)}{N} - \gamma}{\beta \frac{S(t)}{N}} \geq \frac{\beta \rho - \gamma}{\beta \rho}$ of the rate of increase in $C$.
Therefore, since $I(0) = C(0)$, $I(t_\rho) \geq C(t_\rho) \frac{\beta \rho - \gamma}{\beta \rho} = N(1-\rho) \frac{\beta \rho - \gamma}{\beta \rho}$.
\end{proof}

\begin{lemma} \label{lemma2}
% \begin{align}
For $t \in [\tone, \ttwo]$, where $\rho_2 > \rho_1$ for $\rho_1, \rho_2 \in [ 0, \frac{\gamma}{\beta}]$, $\ttwo-\tone \leq \frac{N(\rho_1-\rho_2)}{\beta \rho_2 I(\tone)}$. 
% \end{align}
\end{lemma}
\begin{proof}[Proof of Lemma~\ref{lemma2}]
The difference in $S$ between $\tone$ and $\ttwo$ is $S(\tone) - S(\ttwo) = N(\rho_1 - \rho_2)$. As a consequence of the mean value theorem, $\frac{S(\ttwo) - S(\tone)}{\ttwo - \tone} \leq \max_{t \in [\tone, \ttwo]} \{ \frac{dS}{dt} \}$. Using these two expressions,
% removed --> The difference in $S$ between $\tone$ and $\ttwo$ is $N(\rho_1-\rho_2)$. Then, for all $t \in [\tone, \ttwo]$, 
\begin{align}
\frac{N(\rho_1 - \rho_2)}{\ttwo - \tone} &\geq \min\left\{ -\frac{dS}{dt} \right\} = \min\left\{\beta \frac{S(t)}{N} I(t) : t \in [\tone, \ttwo]\right\} \geq \beta \rho_2 I(\tone)
% removed > \bigg|\frac{dS}{dt}\bigg| \geq \min\left\{\beta \frac{S(t)}{N} I(t) : t \in [\tone, \ttwo]\right\} \geq \beta \rho_2 I(\tone).
\end{align}
The desired expression follows from rearranging terms.
\end{proof}

\begin{lemma} \label{lemma3}
For any $\rho \leq \min\{\frac{\gamma}{\beta}, 1/2\}$,
% \begin{align}
$t_\rho \leq \frac{1}{\beta \rho - \gamma}\log N$.
% \end{align}
\end{lemma}
The proof of this lemma follows the exact same procedure as the proof of Proposition~\ref{prop:T1}. See next section for details.

\begin{proof}[Proof of Proposition~\ref{prop:T2}]
Using the results from Lemmas~\ref{lemma1}-\ref{lemma3},
\begin{align*}
\ttwo 
&= \tone + (\ttwo - \tone) \\
&\leq \frac{1}{\beta \rho_1 - \gamma} \log(\nu N) + \frac{N(\rho_1-\rho_2)}{\beta \rho_2 I(\tone)} \\
&\leq \frac{1}{\beta \rho_1 - \gamma} \log(\nu N) + \frac{(\rho_1-\rho_2) \beta \rho_1}{\beta \rho_2 (1-\rho_1) (\beta\rho_1-\gamma)} \\
&\leq \frac{1}{\beta \rho_1 - \gamma} \log(\nu N) + \frac{C}{(1-\rho_1)},
\end{align*}
where $C = \frac{(1-\rho_2) \beta}{\beta \rho_2 (\beta/2 - \gamma)}$ only depends on $\beta, \gamma$, using the fact that $\rho_1 > 1/2$.
\end{proof}

\subsubsection{Deferred Proofs} % (fold)
\label{sec:deferred_proofs}

\begin{proof}[Proof of Lemma~\ref{lemma3}]
We proceed in the same way as the proof of Proposition~\ref{prop:T1} except in this case we will lower bound $S(0)-S(t)$.

%% removed >
\iffalse
$\tI$ is defined to grow slower than $I$, so it is used as a lower bound.
Define $\tI(t)$ such that $\tI(0) = I(0)$ and $\frac{d\tI}{dt} = (\beta \rho - \gamma) \tI$, implying 
\begin{align}
\tI(t) = I(0) \exp\{ (\beta \rho - \gamma) t\}.
\end{align}
Since $\frac{d\tI}{dt} \leq \frac{dI}{dt}$ when $t < \ttwo$, $\tI(t) \leq I(t)$ for all $t < \ttwo$.

Then, for $t < \ttwo$,
\begin{align}
\frac{dS}{dt} = - \beta \frac{S}{N} I 
              &\leq - \beta \rho \tI.
\end{align}
Hence we can write
\begin{align}
S(t) 
&\leq S(0) +  \int_{0}^{t} - \beta \rho \tI(t') dt' \\
&=S(0)- \beta \rho I(0)\int_{0}^{t}  \exp\{ (\beta \rho - \gamma) t'\} dt' \\
&= S(0)- \frac{\beta \rho I(0)}{\beta \rho - \gamma}( \exp\{ (\beta \rho - \gamma) t \} -1)  \\
\end{align}
\fi
%% removed <

Using the definitions of the deterministic SIR model (with $\beta > \gamma$) and $t_\rho$, for any $\rho \leq \min\{\frac{\gamma}{\beta}, 1/2\}$ and any $t \leq t_\rho$, we write
\begin{align*}
S(t) 
&= S(0) +  \int_{0}^{t} - \beta \frac{S}{N} I(t') dt' \\
&= S(0) +  \int_{0}^{t} - \beta \frac{S}{N} I(0) \exp\{ (\beta \frac{S}{N}  - \gamma) t'\} dt' \\
&\leq S(0)- \beta \rho  I(0) \int_{0}^{t}  \exp\{ (\beta \rho  - \gamma) t'\} dt' \\
&= S(0)- \frac{\beta \rho  I(0)}{\beta \rho  - \gamma}( \exp\{ (\beta \rho - \gamma) t \} -1) 
\end{align*}

Notice we used the fact that for every $t \leq t_\rho$, $S/N$ equals $\rho'$ corresponding to $t$ (i.e. $t_{\rho'}=t$) and hence, $S/N$ is bounded by $\rho$. Since $S(t_\rho) = \rho N$,
\begin{align*}
\rho N &\leq  S(0) - \frac{\beta \rho I(0)}{\beta \rho - \gamma}( \exp\{ (\beta \rho - \gamma) t_\rho \} -1).
\end{align*}
Solving for $t_\rho$ results in
\begin{align}
t_\rho 
 \leq \frac{\log\left(\frac{\beta \rho - \gamma}{\beta \rho I(0)} (S(0) - \rho N) + 1 \right)}{\beta \rho - \gamma} \leq \frac{1}{\beta \rho - \gamma} \log(\nu N)
\end{align}
% Let $\rho_0 = S(0)/N$. Since $I(0) = N - S(0)$ is a constant, $\rho_0 \rightarrow 1$ as $N \rightarrow \infty$.
where $\nu = \frac{2(\beta-\gamma)}{\beta I(0)}$, using the fact that $\rho > 1/2$.
\end{proof}

\subsection{Time to daily infections peak}

Let $T^d_{3,n} = \{t : \frac{d^2S}{dt^2} > 0\}$ be the time at which the rate of new infections is highest.
\begin{theorem}
As $n \rightarrow \infty$, $T^d_{1,n} \leq T^d_{3,n} \leq T^d_{2,n}$.
\end{theorem}

\begin{proof}
\begin{align}
\frac{d^2S}{dt^2}
&= \frac{-\beta}{\pop}\left( \frac{dS}{dt} I + \frac{dI}{dt}S \right) \label{eq:1} \\
&= \frac{-\beta}{\pop}\left( \frac{-\beta S}{\pop} I^2+ \left(\frac{\beta S}{\pop} - \gamma \right)I S \right) \\
&= -\beta IS\left( -\beta I+ \beta S - \gamma \pop  \right)  \\
&= \beta^2 IS\left( I- S + \frac{\gamma}{\beta} \pop  \right) \label{eq:4}
\end{align}
From \eqref{eq:1}, we see that if $\frac{dI}{dt} = 0$, then since $\frac{dS}{dt}<0$, $\frac{d^2S}{dt^2} > 0$.
Therefore, $T^d_{3,n} \leq T^d_{2,n}$.

From \eqref{eq:4}, we see that $\frac{d^2S}{dt^2} > 0$ if and only if
\begin{align} \label{eq:condition}
S <  \frac{\gamma}{\beta} \pop + I.
\end{align}

At $t = T^d_{1,n}$, $C_n(t) = (\pop)^{2/3}$ which implies $I(t) \leq (\pop)^{2/3}$ and $S(t) = \pop - (\pop)^{2/3}$.
We assume $n$ is large enough so that $2(\pop)^{-1/3} < 1- \frac{\gamma}{\beta}$.
Then, \eqref{eq:condition} cannot hold:
\begin{align}
2(\pop)^{-1/3} &< 1- \frac{\gamma}{\beta} \\
\frac{\gamma}{\beta} + (\pop)^{-1/3} &< 1- (\pop)^{-1/3} \\
\frac{\gamma}{\beta} \pop + I < \frac{\gamma}{\beta} \pop + (\pop)^{2/3} &< \pop - (\pop)^{2/3}  = S(t).
\end{align}
Therefore, $T^d_{1,n} \leq T^d_{3,n}$.
\end{proof}
