# Supplementary material for: The Limits to Learning a Diffusion Model
Source: arXiv:2006.06373 source file (2023-05-23)
Supplement: Supplementary file 3 [file peak_condition.tex]

%!TEX root=../SIR-model-EC.tex
In the practical model, $P[t]$ represents the regions that have enough observations to reliably estimate $\alpha$ at time $t$.
In this section, we justify why the definition \eqref{eq:peaks} is a sufficient condition.
Let $t^d_{3} = \inf \{t : \frac{d^2s}{dt^2} > 0\}$ be the time at which the rate of new infections is highest in the deterministic SIR model.
\begin{proposition}
$\lim_{N \rightarrow \infty} t^d_{1} - t^d_{3} \leq 0$.
\end{proposition}

\begin{proof}
\begin{align}
\frac{d^2s}{dt^2}
&= \frac{-\beta}{\pop}\left( \frac{ds}{dt} i + \frac{di}{dt}s \right) \label{eq:1} \\
&= \frac{-\beta}{\pop}\left( \frac{-\beta s}{\pop} i^2+ \left(\frac{\beta s}{\pop} - \gamma \right)i s \right) \\
% &= -\beta is\left( -\beta i+ \beta s - \gamma \pop  \right)  \\
&= \frac{ \beta^2 is}{N^2} \left( i- s + \frac{\gamma}{\beta} \pop  \right) \label{eq:4}
\end{align}
% From \eqref{eq:1}, we see that if $\frac{di}{dt} = 0$, then since $\frac{ds}{dt}<0$, $\frac{d^2s}{dt^2} > 0$.
% Therefore, $T^d_{3,n} \leq T^d_{2,n}$.
From \eqref{eq:4}, we see that $\frac{d^2s}{dt^2} > 0$ if and only if
\begin{align} \label{eq:condition}
s <  \frac{\gamma}{\beta} \pop + i.
\end{align}

At $t \leq t^d_{1}$, $c(t) \leq \pop^{2/3}$ which implies $i(t) \leq \pop^{2/3}$ and $s(t) \geq \pop - \pop^{2/3}$.
We assume $N$ is large enough so that $2(\pop)^{-1/3} < 1- \frac{\gamma}{\beta}$.
Then, \eqref{eq:condition} cannot hold:
\begin{align}
2(\pop)^{-1/3} &< 1- \frac{\gamma}{\beta} \\
\frac{\gamma}{\beta} + (\pop)^{-1/3} &< 1- (\pop)^{-1/3} \\
\frac{\gamma}{\beta} \pop + i(t) \leq \frac{\gamma}{\beta} \pop + (\pop)^{2/3} &< \pop - (\pop)^{2/3}  \leq s(t).
\end{align}
Therefore, $t^d_{1} \leq t^d_{3}$.
\end{proof}
